# Supplementary material for: Writing and storing information in an array of magnetic vortex nanodisks using their azimuthal modes
Source: arXiv:1710.10613 source file (2017-10-29)
Supplement: Supplementary file 1 [file Supplementary_Information.pdf]

# Supplementary information

# Writing and storing information in an array of magnetic vortex nanodisks using the azimuthal modes

H. Vigo-Cotrina

Centro Brasileiro de Pesquisas Físicas, 22290-180, Rio de Janeiro, RJ, Brazil

A.P. Guimarães

Centro Brasileiro de Pesquisas Físicas, 22290-180, Rio de Janeiro, RJ, Brazil

**1) Micromagnetic simulations**

We used the open source software Mumax3 [S1], with discretization cell size of 2 x 2 x L $nm^3$, where L is the thickness of the disk. The material used is Permalloy (NiFe) with typical parameters [S2-S4]: saturation magnetization $M_s$ = 8.6 x $10^5$ A/$m^2$, exchange stiffness A = 1.3 x $10^{-11}$ J/m, and damping constant α = 0.01. The perpendicular uniaxial anisotropy constant $K_z$ varied from 0 to 200 kJ/$m^3$.

**2) Switching times ($t_{sw}$)**

We have obtained the values of the switching times ($t_{sw}$) following the methodology used in references [S5,S6]: the peak shown by the maximum torque indicates the switching of the vortex core. One single peak means a single switching (Fig. 1(a)), two or more peaks means multiple switching (Fig. 1(b)).

The peaks are formed by the abrupt change (vortex-antivortex pairs annihilation) in the magnetization to reverse the vortex core polarity [S5,S6].

In Fig. 2 we show $t_{sw}$ for all values of $K_z$ used in this work.

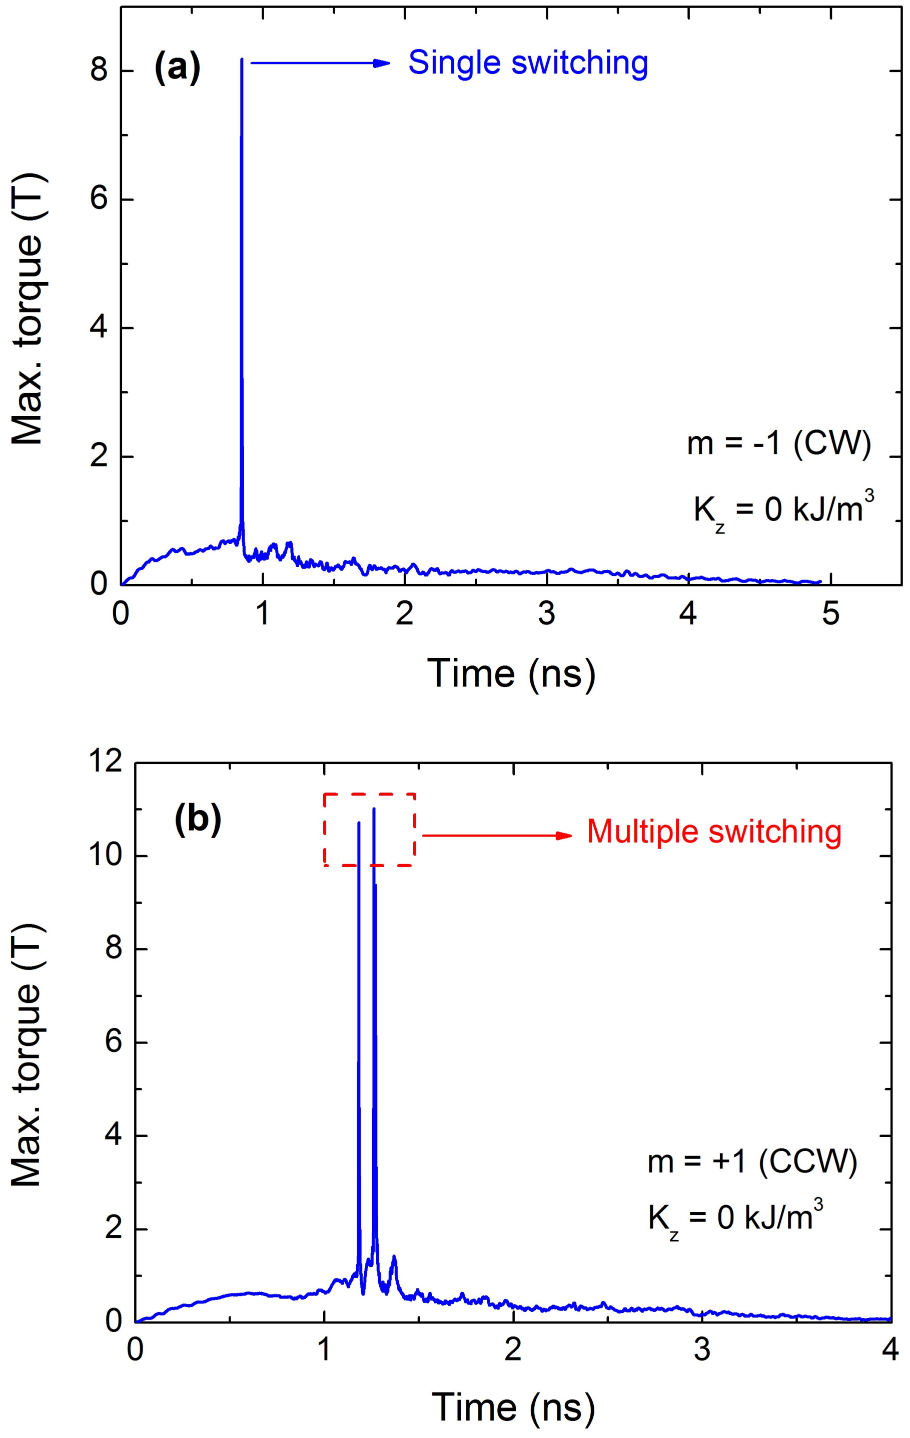


Figure 1: Time dependence of the maximum torque for (a) m = +1 (CCW) and (b) m = -1 (CW) and $K_z$ = 0 kJ/$m^3$.

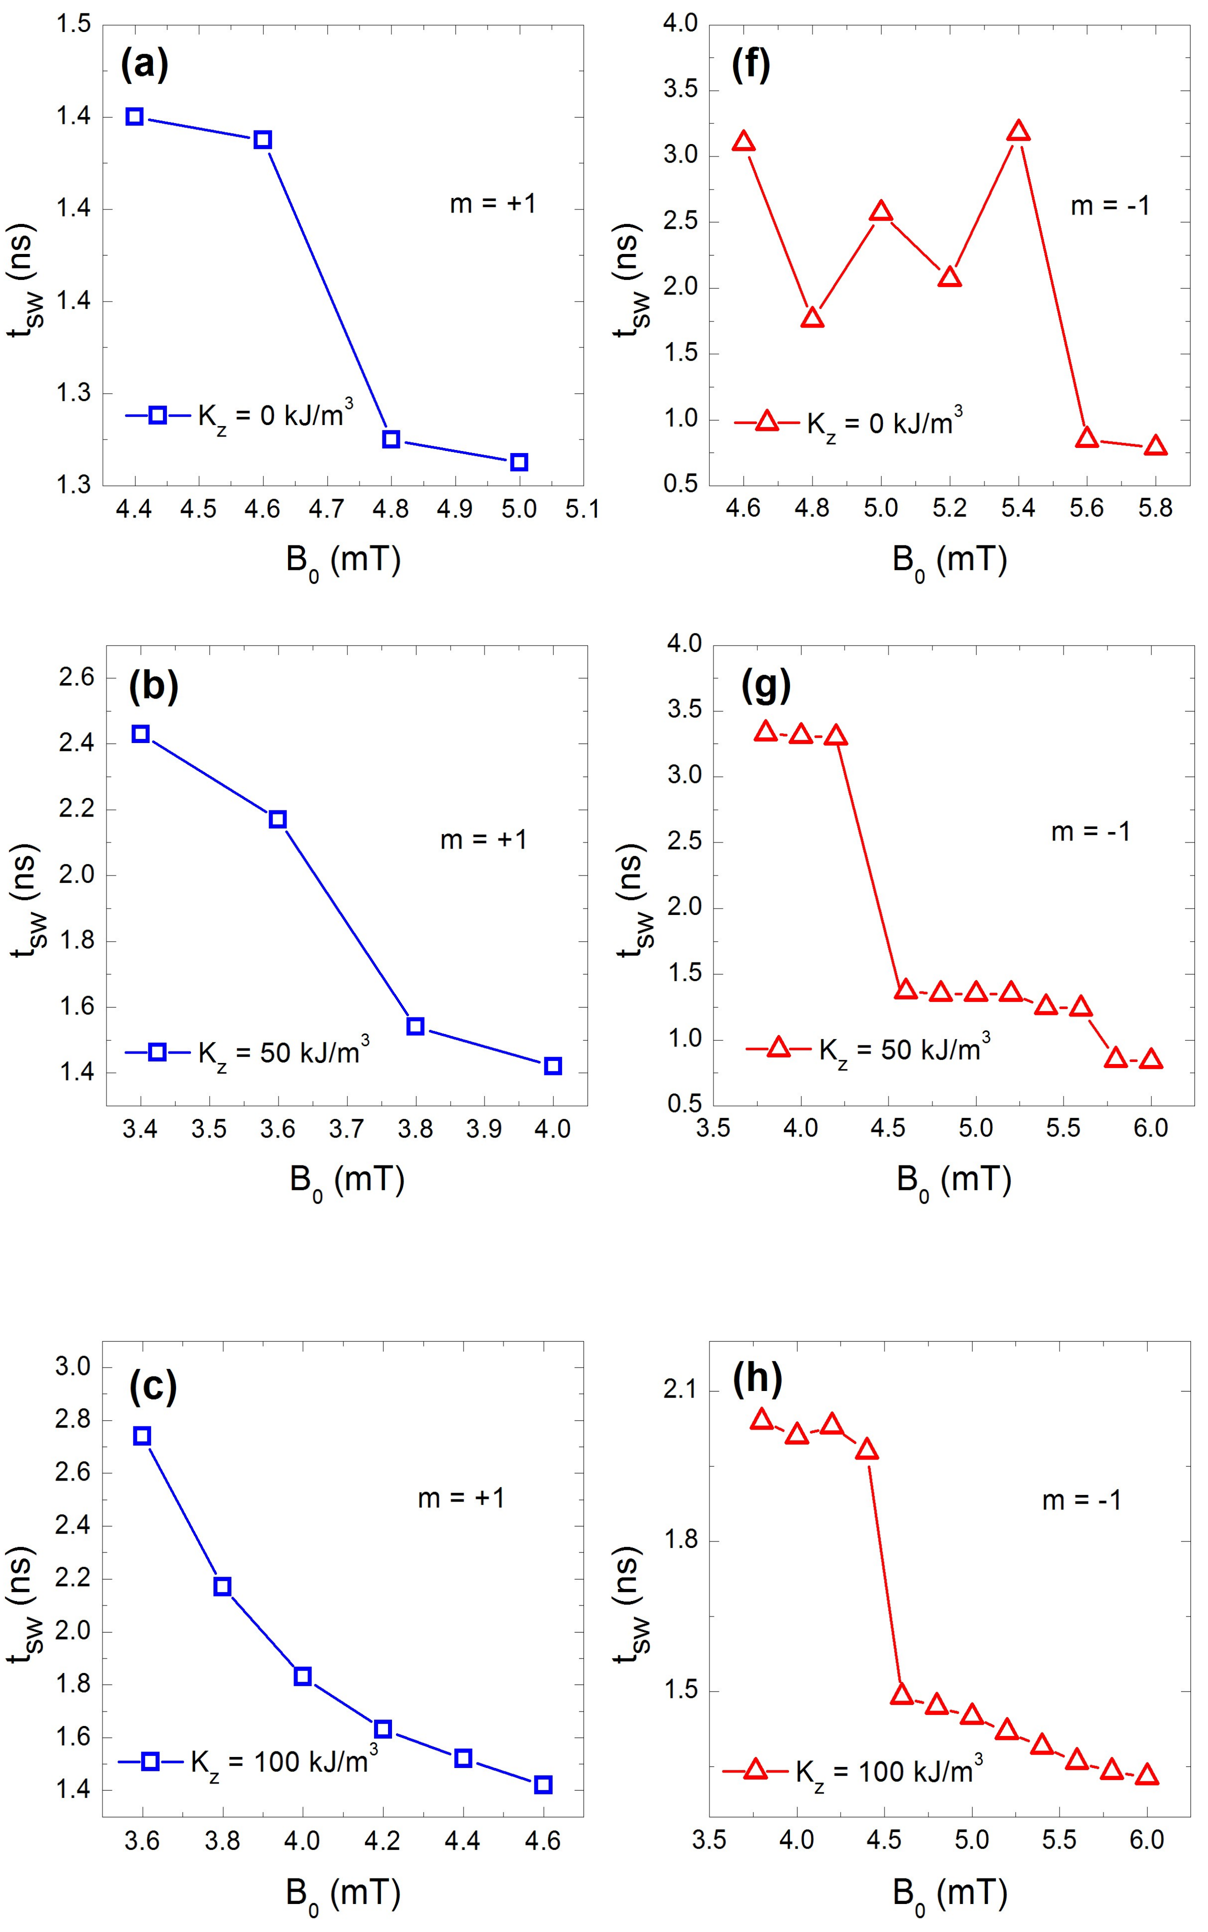
(a)
m = +1
K_z = 0 kJ/m^3
1.5
1.4
1.4
1.4
1.3
1.3
4.4
4.5
4.6
4.7
4.8
4.9
5.0
5.1
t_sw (ns)
B_0 (mT)
(f)
m = -1
K_z = 0 kJ/m^3
4.0
3.5
3.0
2.5
2.0
1.5
1.0
0.5
4.6
4.8
5.0
5.2
5.4
5.6
5.8
t_sw (ns)
B_0 (mT)
(b)
m = +1
K_z = 50 kJ/m^3
2.6
2.4
2.2
2.0
1.8
1.6
1.4
3.4
3.5
3.6
3.7
3.8
3.9
4.0
t_sw (ns)
B_0 (mT)
(g)
m = -1
K_z = 50 kJ/m^3
4.0
3.5
3.0
2.5
2.0
1.5
1.0
0.5
3.5
4.0
4.5
5.0
5.5
6.0
t_sw (ns)
B_0 (mT)
(c)
m = +1
K_z = 100 kJ/m^3
3.0
2.8
2.6
2.4
2.2
2.0
1.8
1.6
1.4
3.6
3.8
4.0
4.2
4.4
4.6
t_sw (ns)
B_0 (mT)
(h)
m = -1
K_z = 100 kJ/m^3
2.1
1.8
1.5
3.5
4.0
4.5
5.0
5.5
6.0
t_sw (ns)
B_0 (mT)

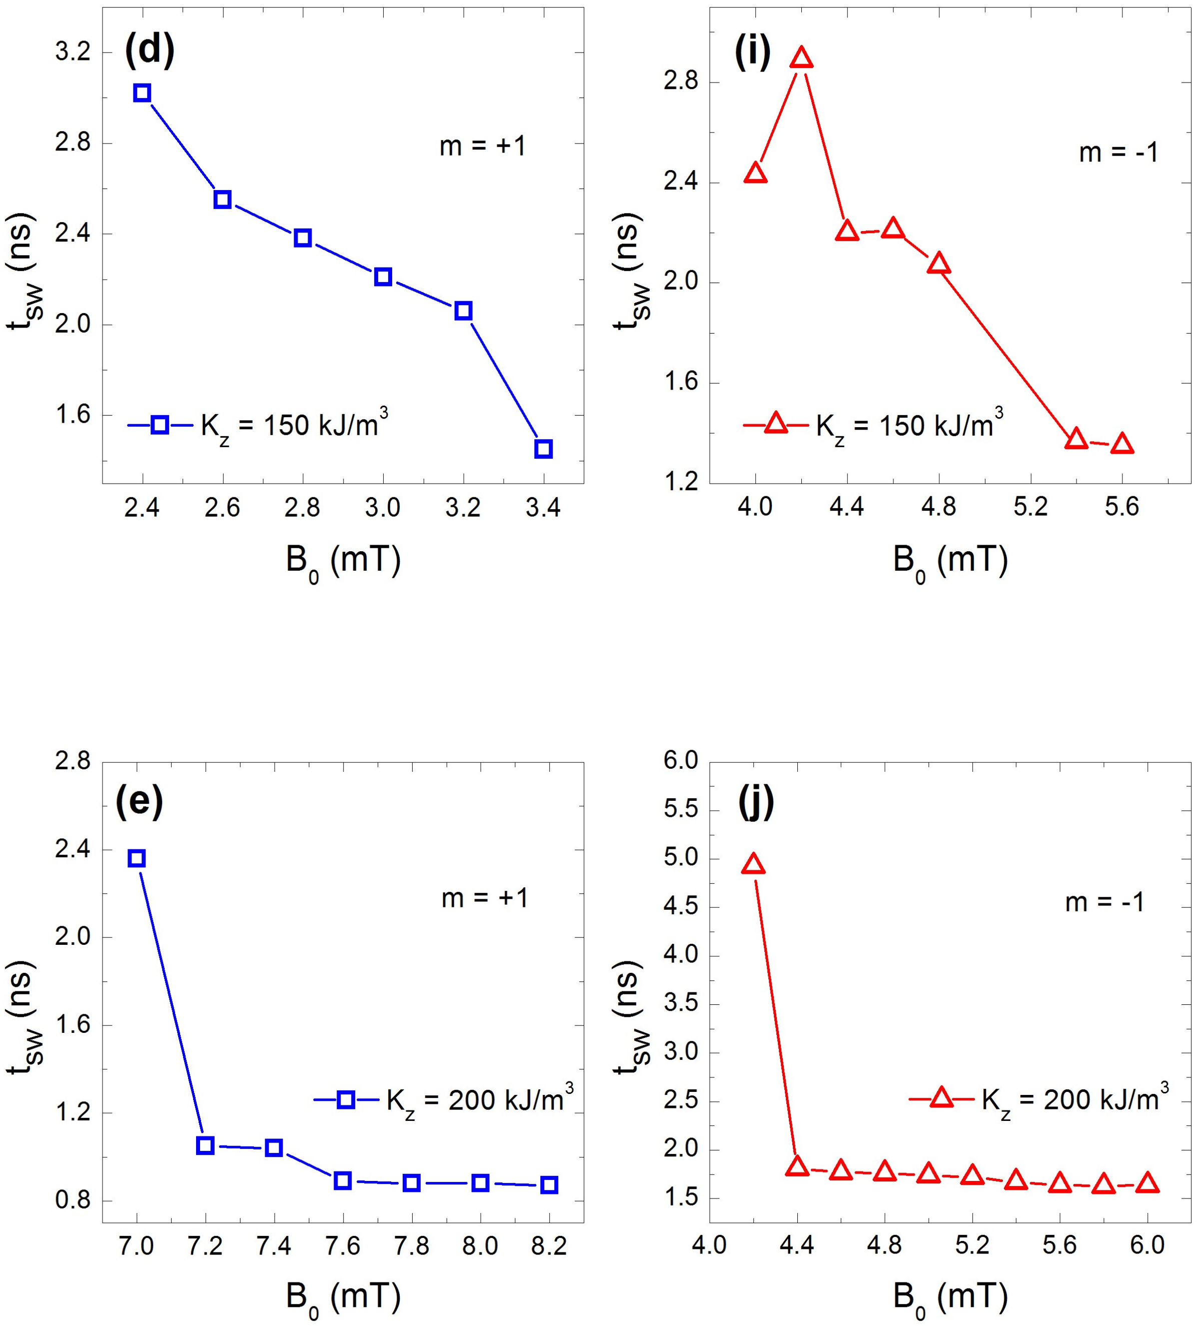


Fig. 2: Switching times versus magnetic field intensity for (a-e) m = +1 (CCW) and (f-j) m = -1 (CW) for different values of $K_z$.

**3) References**


**[S1]** A. Vansteenkiste, J. Leliaert, M. Dvornik, M. Helsen, F. Garcia-Sanchez, B. Van Waeyenberge, The design and verification of Mumax3, AIP Advances 4 (2014) 107133. doi:10.1063/1.4899186.

**[S2]** K. Y. Guslienko, Magnetic vortex state stability, reversal and dynamics in restricted geometries, J. Nanosc. Nanotech. 8 (2008) 2745–2760. doi:10.1166/jnn.2008.003.

**[S3]** E. R. P. Novais, S. Allende, D. Altbir, P. Landeros, F. Garcia, A. P. Guimarães, Effect of perpendicular uniaxial anisotropy on the annihilation fields of magnetic vortices, J. Appl. Phys. 114 (15) (2013). doi:10.1063/1.4824803.

**[S4]** K. Y. Guslienko, B. A. Ivanov, V. Novosad, Y. Otani, H. Shima, K. Fukamichi, Eigenfrequencies of vortex state excitations in magnetic submicron-size disks, J. Appl. Phys. 91 (2002) 8037–8039. doi:10.1063/1.1450816.

**[S5]** Q. F. Xiao, J. Rudge, and B. C. Choi, Dynamics of vortex core switching in ferromagnetic nanodisks, Appl. Phys. Lett. 89, 262507 (2006). doi: 10.1063/1.2424673

**[S6]** Matthias Kammerer, Hermann Stoll, Matthias Noske, Markus Sproll, Markus Weigand, Christian Illg, Georg Woltersdorf, Manfred Fähnle, Christian Back, and Gisela Schütz, Fast spin-wave-mediated magnetic vortex core reversal, Phys. Rev. B 86, 134426 (2012). doi: 10.1103/PhysRevB.86.134426
